# Supplementary material for: Long-time predictive modeling of nonlinear dynamical systems using neural networks
Source: arXiv:1805.12547 source file (2018-11-14)
Supplement: Supplementary file 1 [file appendix.tex]

\appendix
%\section{Generation of data}{\label{apdx:dataGen}}
%
%This section describes the details of generating data in this work. In this work we will have two different configurations of generating data. First one is generating data of a single trajectory. Second one is generating feature-target pair with feature randomly selected in feature space. Following corresponding equation of discrete dynamics, we generate training data and testing data based on parameters in the Table followed.

\section{Proper orthogonal decomposition (POD) and shift-mode}
{\label{apd:pod}}

Proper orthogonal decomposition (POD) is also closely related to the singular value decomposition (SVD), principle component analysis (PCA), Karhunen-Lo\`eve (KL) expansion of a spatial temporal field $\bm{u}(\bm{x},t)$. Usually, we consider a finite truncation of the expansion to approximate $\bm{u}(\bm{x},t)$ in the `energy' or variance sense.
\begin{equation}
\bm{u}(\bm{x},t) \approx \bm{u}^{[N]} = \bm{u}_0(\bm{x}) + \sum_{i=1}^N  a_i(t)\bm{u}_i(\bm{x}),
\end{equation}
where $\bm{u}(\bm{x},t) \in \mathbb{R}^3$, $\bm{x} \in \mathbb{R}^3$, $\bm{u}_0$ is the mean flow, while $\{ \bm{u}_i \}_{i=1}^{N}$ are the first $N$ KL modes and $a_i$ is time-dependent coefficients which can be determined uniquely by orthogonal projection in a Hilbert space endowed with the inner product $\langle \bm{v}, \bm{w}\rangle = \int_{\Omega} dA \bm{v} \cdot \bm{w}$.
